# Supplementary material for: FDR-Corrected Sparse Canonical Correlation Analysis with Applications to Imaging Genomics
Source: arXiv:1705.04312 ancillary file (2018-06-23)
Supplement: Supplementary file 1 [file FDRcorrectedSCCA_supplementary_materials.pdf]

# Supplementary Materials for: "FDR-Corrected Sparse Canonical Correlation Analysis with Applications to Imaging Genomics"

Alexej Gossmann, Pascal Zille, Vince Calhoun, and Yu-Ping Wang

## I. Simulation study on low-dimensional Gaussian data

In the low-dimensional case we have performed simulations analogous to the ones presented in Section V-A of the main text, with the difference that $n = 3000$, $p_X = p_Y = 50$, and $s_X, s_Y \in \{1, 10, 20, 30\}$. Moreover, since the problem is already low-dimensional, the sparsity of the preliminary solution $\widehat{\mathbf{u}}^{(0)}$ and $\widehat{\mathbf{v}}^{(0)}$ does not need to be restricted in Step 2 of Procedure 1. Therefore we obtain the preliminary estimates via the conventional $\ell_1$ penalized CCA of Equation (2) with $c_1 = c_2 = 0.9 \cdot \sqrt{p_X}$, which generally yields dense preliminary estimates $\widehat{\mathbf{u}}^{(0)}$ and $\widehat{\mathbf{v}}^{(0)}$ under the considered simulation settings. The proposed FDR-corrected sparse CCA procedure is compared to several other widely-used sparse CCA methods – the same methods as the ones considered in Section V-A. Analogously to Section V-A, for each of the considered methods we report the estimated FDR in Figures 1a and 1b, and the estimated TPR in Figures 1c and 1d. While in Section V-A we reported only $\mathrm{FDR}(\widehat{\mathbf{v}})$ and $\mathrm{TPR}(\widehat{\mathbf{v}})$, and did not include analogous figures for $\mathrm{FDR}(\widehat{\mathbf{u}})$ and $\mathrm{TPR}(\widehat{\mathbf{u}})$ due to space constraints, here we include results for both $\widehat{\mathbf{u}}$ and $\widehat{\mathbf{v}}$. In particular, it is evident that the FDR-corrected sparse CCA procedure as well as all other considered sparse CCA methods treat the two canonical vectors $\mathbf{u}$ and $\mathbf{v}$ equally, resulting in estimated FDR and TPR values that are very close to each other under analogous settings for $\mathbf{u}$ and $\mathbf{v}$. As one can expect from a statistical method, our sparse CCA procedure performs better in terms of both FDR and TPR on low-dimensional data ($n \ll p_X, p_Y$) considered here, than on high-dimensional data ($n \gg p_X, p_Y$), which is the case considered in Section V-A. Here, the FDR of our method is always below the nominal level $q$, but closer to the nominal level than in the high-dimensional scenarios, and the TPR of our method is approximately equal to 1 under all but the most sparse conditions ($s_X = s_Y = 1$). Similarly to what is discussed in Section V-A about the simulation studies with high-dimensional data, our FDR-corrected sparse CCA procedure generally outperforms the competing sparse CCA methods in terms of the considered FDR and TPR criteria when applied to low-dimensional data as well, by achieving $\mathrm{TPR} \approx 1$ under all settings but the sparsest one ($s_X = s_Y = 1$) while always maintaining an FDR below the nominal level $q$ without being too conservative.

## II. Exploratory analysis for potentially confounding factors in PNC

Section VI-A of the main text discusses an exploratory analysis that we have performed in order to investigate whether factors, such as ethnicity, genotyping platform, or age of the subjects, can confound the CCA analysis of the Philadelphia Neurodevelopmental Cohort (PNC, [3]) data, which is presented in Section VI-B. For the performed exploratory analysis we mostly considered principle component analysis (PCA) based techniques, such as the ones discussed in [4], [5], which are aimed at identifying population stratification, batch effects, or other confounding factors. The results are discussed in Section VI-A of the main text, while the main text omits the relevant visualizations due to space constraints. These are supplemented here in form of Figures 2a, 2b, and 2c. We applied PCA to the data matrices (the matrices $X$ and $Y$ from the PNC analysis of Section VI-B), and plotted the subject-specific loadings corresponding to the first few components against each other. For the genomic data (see Section VI), a systematic separations of different ethnicities by some of the principle components is evident, but there seems to be no influence by other factors, including the genotyping platform, subjects' gender, or age (see Figure 2a). For the brain connectivity data (see Section VI), there do not seem to be systematic differences or grouping with respect to ethnicity, genotyping platform, or gender (see Figure 2b). However some of the first few brain connectivity specific principle components seem to vary with the subjects' age (see Figure 2c).

## Acknowledgment

The work was partially supported by NIH (R01 GM109068, R01 MH104680, R01 MH107354, P20 GM103472, R01 REB020407, 1R01 EB006841) and NSF (#1539067).

## References

[1] D. M. Witten, R. Tibshirani, and T. Hastie, "A penalized matrix decomposition, with applications to sparse principal components and canonical correlation analysis," *Biostatistics*, vol. 10, no. 3, pp. 515–534, Jul. 2009.

[2] E. Parkhomenko, D. Tritchler, and J. Beyene, "Sparse canonical correlation analysis with application to genomic data integration," *Statistical applications in genetics and molecular biology*, vol. 8, 6 Jan. 2009.

[3] T. D. Satterthwaite, M. A. Elliott, K. Ruparel, J. Loughead, K. Prabhakaran, M. E. Calkins, R. Hopson, C. Jackson, J. Keefe, M. Riley *et al.*, "Neuroimaging of the Philadelphia neurodevelopmental cohort," *NeuroImage*, vol. 86, pp. 544–553, 1 Feb. 2014.

[4] A. L. Price, N. J. Patterson, R. M. Plenge, M. E. Weinblatt, N. A. Shadick, and D. Reich, "Principal components analysis corrects for stratification in genome-wide association studies," *Nature genetics*, vol. 38, no. 8, pp. 904–909, Aug. 2006. [Online]. Available: http://dx.doi.org/10.1038/ng1847

[5] J. T. Leek, R. B. Scharpf, H. C. Bravo, D. Simcha, B. Langmead, W. E. Johnson, D. Geman, K. Baggerly, and R. A. Irizarry, "Tackling the widespread and critical impact of batch effects in high-throughput data," *Nature reviews. Genetics*, vol. 11, no. 10, pp. 733–739, Oct. 2010. [Online]. Available: http://dx.doi.org/10.1038/nrg2825

A. Gossmann is with the Bioinnovation PhD Program, Tulane University, New Orleans, LA. Web: http://www.alexejgossmann.com.

Y.-P. Wang and P. Zille are with the Department of Biomedical Engineering, Tulane University, New Orleans, LA.

V. Calhoun is with The Mind Research Network, and the Department of Electrical and Computer Engineering, University of New Mexico, Albuquerque, NM.

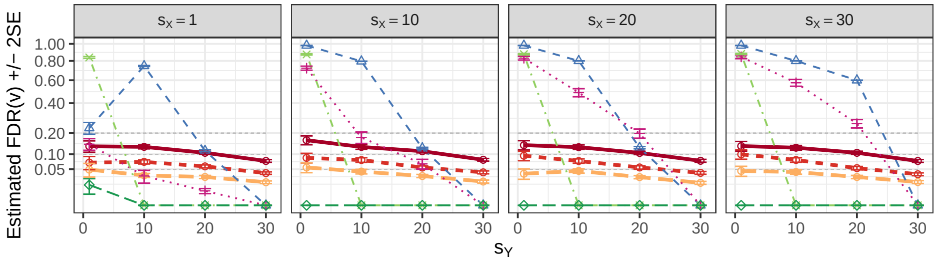


(a) Estimated FDR $(\widehat{\mathbf{v}})$ by true sparsity of $\mathbf{u}$ and $\mathbf{v}$.

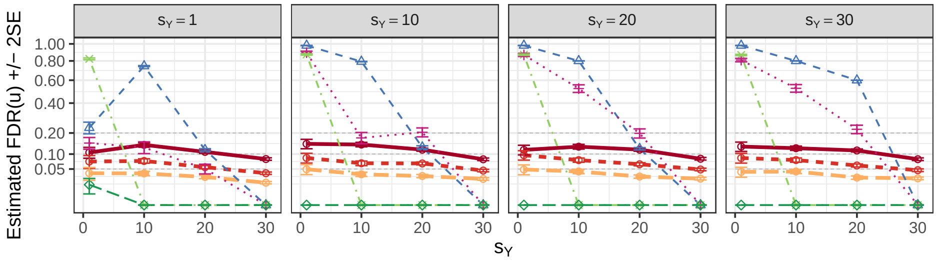


(b) Estimated FDR $(\widehat{\mathbf{u}})$ by true sparsity of $\mathbf{u}$ and $\mathbf{v}$.

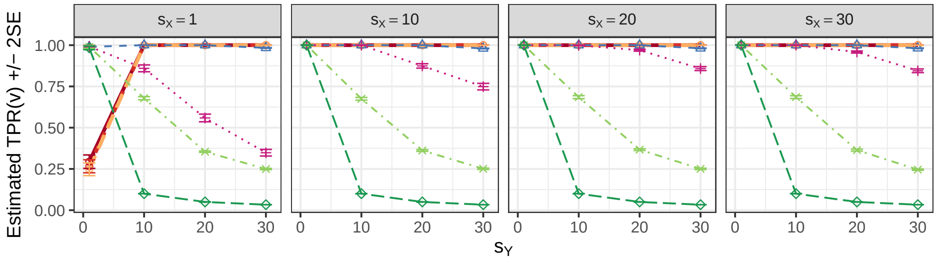


(c) Estimated TPR $(\widehat{\mathbf{v}})$ (sensitivity) by true sparsity of $\mathbf{u}$ and $\mathbf{v}$.

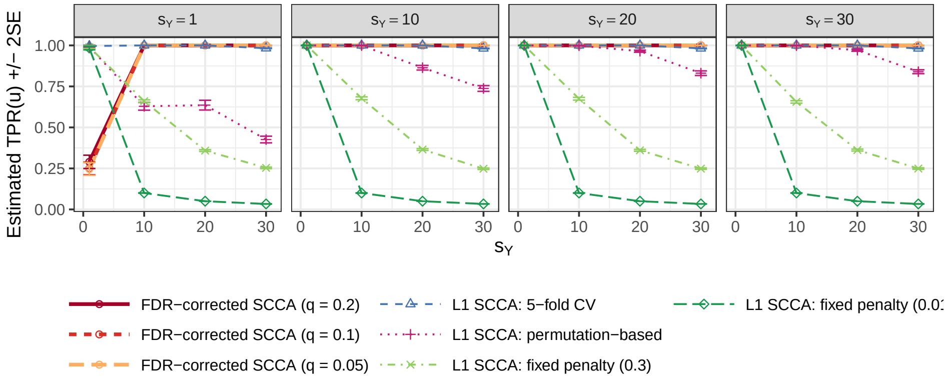


(d) Estimated TPR $(\widehat{\mathbf{u}})$ (sensitivity) by true sparsity of $\mathbf{u}$ and $\mathbf{v}$.

Fig. 1. The performance of the proposed FDR-corrected sparse CCA procedure, at different target FDR levels $q = 0.05, 0.1, 0.2$ is compared to the $\ell_1$-penalized sparse CCA (L1 SCCA) with the penalty parameters either set to a fixed value (high sparsity: $\lambda = 0.01$, or moderate sparsity: $\lambda = 0.3$), or selected via the permutation based method of [1], or selected via a 5-fold cross-validation procedure (an approach based on [2]). The matrices $X, Y \in \mathbb{R}^{3000\times 50}$ have Gaussian entries. All values are averaged over 500 simulation runs performed at each combination of parameters, and all error bars correspond to $\pm$2SE. (a) The estimated false discovery rate (FDR) in $\widehat{\mathbf{v}}$ is shown (on a square root scale) with respect to changes in $s_X$, the number of nonzero entries of $\mathbf{u}$, and $s_Y$, the number of non-zero entries of $\mathbf{v}$. The estimated FDR of the proposed FDR-corrected sparse CCA procedure always stays below the specified upper bound $q$. Estimated FDR of every other method among the considered is generally not adaptive to changes in $s_X$ and $s_Y$. (b) An analogous plot to (a) showing the estimated FDR in $\widehat{\mathbf{u}}$. Each method's estimator of $\mathbf{u}$ shows exactly the same behaviour as the corresponding estimator of $\mathbf{v}$. (c) The estimated true positive rate (TPR, or sensitivity) of $\widehat{\mathbf{v}}$ is shown with respect to changes in $s_X$ and $s_Y$. The FDR-corrected sparse CCA procedure has very good TPR compared with the other methods, even though its FDR behavior is much better than that of other methods (i.e., controlled at a fixed level $q$). (d) An analogous plot to (c) showing the estimated TPR in $\widehat{\mathbf{u}}$. The estimators of $\mathbf{u}$ show exactly the same behavior as those of $\mathbf{v}$.

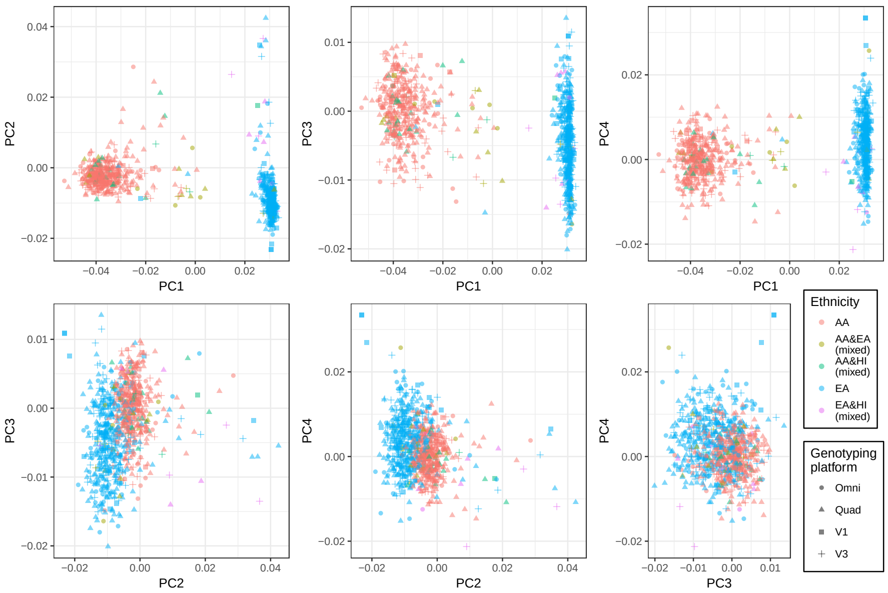


(a) PCA of the genomic data

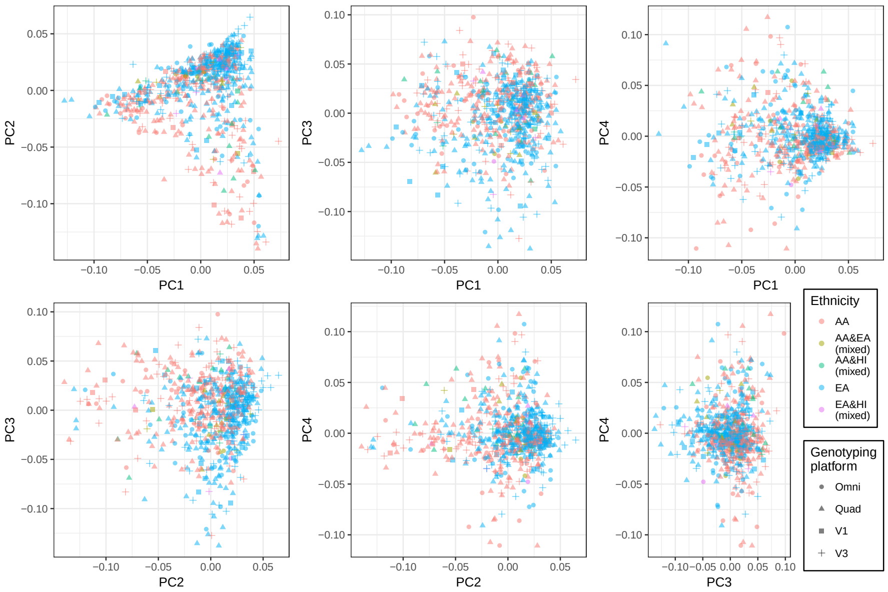


(b) PCA of the brain connectivity data

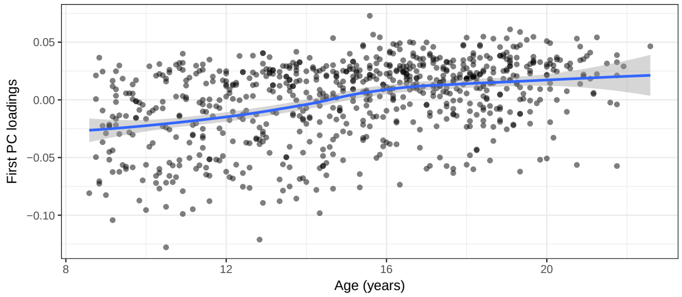


(c) First PC of the brain connectivity data by age

Fig. 2. (a) PCA is applied to the genomic data, the matrix $X$ from the PNC analysis of Section VI-B. The subject-specific loadings corresponding to the first four components are shown plotted against each other. A systematic separations of different ethnicities by some of the principle components is evident. Genotyping platform differences do not seem to have an influence, and likewise no influence of gender or age (not shown) has been observed. (b) PCA is applied to the matrix of brain functional connectivity measures, $Y$ from the PNC analysis of Section VI-B. The subject-specific loadings corresponding to the first four components are shown plotted against each other. No systematic differences or grouping with respect to ethnicity, genotyping platform, or gender (gender not shown) are evident. However, (c) a portion of the variability in some of the first few brain specific principle components can be explained by the subjects' age (shown are the subject specific loadings corresponding to the first principle component). [*Abbreviations.* AA: Black or African American; EA: European American; HI: Hispanic/Latino; Omni: Illumina Omni Array; Quad: Illumina Human610; V1: Illumina HumanHap550v1; V3: Illumina HumanHap550v3.]
